# Supplementary material for: Bialgebraic Reasoning on Stateful Languages
Source: arXiv:2503.10955 source file (2025-07-21)
Supplement: Supplementary file 1 [file additional-macros.tex]

%
%

\DeclareMathSymbol{\mathinvertedexclamationmark}{\mathord}{operators}{'074}
\DeclareMathSymbol{\mathexclamationmark}{\mathord}{operators}{'041}
\makeatletter
\newcommand{\raisedmathinvertedexclamationmark}{%
  \mathord{\mathpalette\raised@mathinvertedexclamationmark\relax}%
}
\newcommand{\raised@mathinvertedexclamationmark}[2]{%
  \raisebox{\depth}{$\m@th#1\mathinvertedexclamationmark$}%
}
\makeatother

\newcommand{\longTo}{\Longrightarrow}
\newcommand{\Pt}{V}
\newcommand{\R}{\mathcal{R}}
\newcommand{\st}{\mathsf{st}}
\newcommand{\lsmc}{\fatsemi}
\newcommand{\Pre}{\mathbf{Pre}}
\newcommand{\Pow}{\mathcal{P}}
\newcommand{\xTo}{\xRightarrow}
\makeatletter
\renewcommand\xRightarrow[2][]{
  \ifx\relax#1\relax%
    \ext@arrow 0055{\Rightarrowfill@}{}{#2\ }
  \else%
    \ext@arrow 0055{\Rightarrowfill@}{#1\ }{#2\ }
  \fi
}
\makeatother
\newcommand{\HJBis}{\mathbf{HJBisim}}
\newcommand{\Bis}{\mathbf{Bisim}}
\newcommand{\primrec}{\mathsf{pr}\,}
\newcommand{\hattau}{\hat{\tau}}
\newcommand{\hatr}{\hat{r}}
\newcommand{\hatbeta}{\hat{\beta}}
\newcommand{\lft}{{\mathsf{l}}}
\newcommand{\rgt}{{\mathsf{r}}}
\newcommand{\colim}{\mathsf{colim}}
\newcommand{\terminal}{\mathexclamationmark}
\newcommand{\initial}{\raisedmathinvertedexclamationmark}
\newcommand{\smc}{\mathbin{;}}
\newcommand{\hatR}{{\widehat{R}}}
\newcommand{\qand}{\quad\text{and}\quad}
\newcommand{\qqand}{\qquad\text{and}\qquad}
\newcommand{\rsto}{\rightsquigarrow}
\newcommand{\pb}[2]{\scalebox{#1}{\rotatebox{#2}{$\ulcorner$}}}
\newcommand{\deq}[1]{{\rotatebox{#1}{$=$}}}
\newcommand{\dleq}[1]{{\rotatebox{#1}{$\preceq$}}}
\newcommand{\dgeq}[1]{{\rotatebox{#1}{$\succeq$}}}
\newcommand{\cev}[1]{\reflectbox{\ensuremath{\vec{\reflectbox{\ensuremath{#1}}}}}}
\newcommand{\diag}{\mathsf{in}}
\newcommand{\HO}{\mathcal{HO}}
\newcommand{\Refl}{\mathbf{Refl}}
\newcommand{\Gra}{\mathbf{Gra}}
\newcommand{\RGra}{\mathbf{RGra}}
\newcommand{\RRel}{\mathbf{RRel}}
\newcommand{\happrox}{\mathrel{\hat\lessapprox}}
\newcommand{\happroxs}{\mathrel{\hat\approx^{\star}}}
\newcommand{\under}[1]{\lvert#1\rvert}
\newcommand{\SKI}{\mathrm{SKI}}
\renewcommand{\L}{\mathcal{L}}
\newcommand{\ap}{{\mathrm{ap}}}
\newcommand{\var}{\mathsf{var}}
\newcommand{\cn}{{\mathrm{cn}}}
\newcommand{\cv}{{\mathrm{cv}}}
%
%
\newcommand{\Powf}{\mathcal{P}_{\omega}}
\newcommand{\FSigma}{{\mathbb{\Sigma}}}
\newcommand{\FSigmas}{{\mathbb{\Sigma}}^\star}
\newcommand{\Sigmas}{\Sigma^{\star}}
\newcommand{\FDelta}{{\mathbb{\Delta}}}
\newcommand{\FDeltas}{{\mathbb{\Delta}}^\star}
\newcommand{\ar}{\mathsf{ar}}
%
\newcommand{\NT}{\mathrm{Nat}}
\newcommand{\supp}{\mathsf{supp}}
\newcommand{\epito}{\twoheadrightarrow}
\newcommand{\abs}{\mathsf{abs}}
\newcommand{\conc}{\mathsf{conc}}
\newcommand{\T}{{\mathcal{T}}}
\renewcommand{\S}{{\mathcal{S}}}
\newcommand{\can}{\mathsf{can}}
\newcommand{\lab}{\mathsf{label}}
\newcommand{\leaves}{\mathsf{leaves}}
\newcommand{\incl}{\mathsf{in}}
\newcommand{\seq}{\subseteq}
\newcommand{\ol}{\overline}
\newcommand{\out}{\mathsf{out}}
\newcommand{\outl}{\mathsf{l}}
\newcommand{\outr}{\mathsf{r}}
\newcommand{\trc}{{\mathsf{trc}}}
\newcommand{\fn}{{\mathsf{fn}}}
\newcommand{\beh}{{\mathsf{beh}}}
\providecommand{\C}{}
\providecommand{\D}{}
\providecommand{\E}{}
\renewcommand{\C}{{\mathbb{C}}}
\renewcommand{\D}{{\mathbb{D}}}
\renewcommand{\E}{{\mathbb{E}}}
\renewcommand{\id}{{\mathsf{id}}}
\newcommand{\Nat}{\mathds{N}}
\renewcommand{\NT}{\mathsf{Nat}}

%
%
\newcommand{\stimes}[1]{{S\product #1}}
\newcommand{\xtimes}[1]{{X\product #1}}
\newcommand{\ytimes}[1]{{Y\product #1}}
\newcommand{\sbrks}[1]{{ \brks{\fst,#1}  }}
\newcommand{\cpair}[2]{{ #1, #2 }}
\newcommand{\tpair}[2]{{ #1 \product #2 }}


%
%
%
\renewcommand{\brack}[1]{\lbrack #1 \rbrack}
%
\newcommand{\sbrack}[1]{\llbracket #1 \rrbracket}
%
\newcommand{\ssbrack}[1]{\llbracket\mkern-4.7mu\llbracket #1 \rrbracket\mkern-4.7mu\rrbracket}
%
\newcommand{\f}{\oname{f}}
\newcommand{\fii}{\oname{f}}
%

%
\newcommand{\takeout}[1]{\empty}

\newcommand{\ini}{\iota}
\newcommand{\ter}{\tau}
\newcommand{\wh}{\widehat}
\DeclareMathOperator{\Coalg}{\mathsf{Coalg}}
\DeclareMathOperator{\Alg}{\mathbf{Alg}}
%
\newcommand{\cofun}{(\overline{\rule{-1pt}{7pt}\argument})}
\renewcommand{\rho}{\varrho}
\newcommand{\N}{\mathds{N}}
\newcommand{\opp}{\mathsf{op}}
\newcommand{\xla}[1]{\xleftarrow{~#1~}}
\newcommand{\mypowfin}{\mathscr{P}_\omega}

%
\newcommand{\pullbackangle}[2][]{\arrow[phantom,to path={
                     -- ($ (\tikztostart)!1cm!#2:([xshift=8cm]\tikztostart) $)
                        node[anchor=west,pos=0.0,rotate=#2,
                        inner xsep = 0]
                        {\begin{tikzpicture}[minimum
                        height=1mm,baseline=0,#1]
    \draw[-] (0,0) -- (.5em,.5em) -- (0,1em);
                        \end{tikzpicture}}}]{}}

%
%
%
%
